# Supplementary material for: MSeg: A Composite Dataset for Multi-domain Semantic Segmentation
Source: arXiv:2112.13762 source file (2021-12-27)
Supplement: Supplementary file 1 [file appendix.tex]

 
 
 















% \section{ScanNet Full-Resolution Results}
% \subsection{Joint Model tested on ScanNet-20}

% Please refer to Table \ref{tab:scannet20results}

% \begin{table}[!h]
% \center
% \begin{adjustbox}{max width=\columnwidth}
%     \begin{tabular}{@{}lccc@{}}
%     \toprule
%       \textsc{\textbf{Method + Training Taxonomy}} &   \textsc{\textbf{mIoU}} &  \textbf{mAcc} &   \textsc{\textbf{Acc}} \\
%      \midrule
%          \textsc{ILC-PSPNet}  & 47.5 & & \\
%         \textsc{ENet} \cite{Paszke:Arxiv2016:ENet}  & 37.6 & & 
%       \vspace{2mm} \\
%       \vspace{2mm} \\
%         \textsc{ZS, Naive Taxonomy}  & 39.5 & &  
%       \vspace{2mm} \\
%       \textsc{ZS, MTurk Relabeled Taxonomy} & ??? & &  
%       \vspace{2mm} \\
%       \textsc{ZS, MTurk Relabeled Taxonomy} & & &  \\
%       \textsc{Self-training, Relabeled Taxonomy}  & ??? & & \\
%       \bottomrule
%     \end{tabular}
% \end{adjustbox}
% \caption{Results of 2D, RGB-only methods on the test split of the ScanNet Dataset. \textit{ZS} denotes zero-shot methods, whereas all other methods employ \textit{self-training}. We submit multi-scale predictions for the ScanNet-20 semantic label test benchmark \url{http://kaldir.vc.in.tum.de/scannet_benchmark/semantic_label_2d}. Note that all other methods on the benchmark utilize depth/3D geometry; accordingly, we exclude them for a fair comparison.}
% \label{tab:scannet20results}
% \end{table}


% \section{Ablation of Effects of Individual Datasets}
% \begin{table}[]
%     \centering
%     \begin{tabular}{c|c}
%         All 7 Datasets &  \\
%         7 minus COCO & \\
%         7 minus ADE20K & \\
%         7 minus BDD100K & 
%     \end{tabular}
%     \caption{Intermediate Steps. All of the datasets need to be there. Impact of removing datasets from our group. }
%     \label{tab:my_label}
% \end{table}


% \section{Per-Class Performance with data increases}

% \begin{figure}[!h]
%     \centering
%     \includegraphics[width=\linewidth]{imgs/iou_as_fn_of_training_examples_placeholder.png}
%     \caption{\textcolor{red}{PLACEHOLDER:} We demonstrate how providing a network with additional training data leads to  \ozan{is this figure a placeholder or is it an actual result?}}
%     \label{fig:my_label}
% \end{figure}






% \begin{figure}
%     \centering
%         \begin{tabular}{c@{\hspace{2mm}}c}
%     \includegraphics[width=0.32\columnwidth]{imgs/ADE_val_00000890.jpg} & \includegraphics[width=0.65\columnwidth]{imgs/ade20k_bar_examples.jpg} \\
%     (a) & (b)
%     \end{tabular}
%      \begin{tabular}{c@{\hspace{2mm}}c}
%     \includegraphics[width=0.48\columnwidth]{imgs/ADE_val_00000226_qvga_pred_labels_palette.png} & \includegraphics[width=0.48\columnwidth]{imgs/ADE_val_00000228_qvga_pred_labels_palette.png} \\
%     (c) & (d)
%     \end{tabular}
%     \begin{tabular}{c@{\hspace{2mm}}c@{\hspace{2mm}}c}
%       \includegraphics[width=0.32\columnwidth]{imgs/nyu_val_371_rgb.jpg} &
%       \includegraphics[width=0.31\columnwidth]{imgs/3300_scannet-25k-benchmark_artifact1.png} &
%     \includegraphics[width=0.31\columnwidth]{imgs/800_scannet-25k-benchmark_artifact2.png} \\
%     (e) & (f) & (g)
%     \end{tabular}

%     \caption{Labeling errors are highly prevalent in modern datasets; we resolve many of these problems in MSeg. ADE20K: Road labeled as ``earth'' in (a), Ground labeled as ``floor'' in (c). Pavement labeled as ``floor'' in (d). ADE20K labels counters as restaurants and long metal rods both as ``bar'' in (b), defying taxonomy inter-operability. Accordingly, we ``unlabel'' the ``bar'' mask annotations. ScanNet: boundary artifacts visible on doors in (f,g), (label map superimposed onto RGB image). NYU Depth v2: labels all pixels in the upper left quadrant as bookshelf, rather than as book in (e).  \ozan{Figure is not serving a single purpose, it is either serving too many purposes or no purpose. I am not actually sure which one since I do not understand the section in general}}
%     \label{fig:datasetselferrors}
% \end{figure}




% \begin{figure}
%     \centering
%     \begin{tabular}{c@{\hspace{2mm}}c@{\hspace{2mm}}c}
%         \includegraphics[width=0.31\linewidth]{imgs/ADE_val_00000289_qvga_pred_labels_palette.png}
%         & \includegraphics[width=0.31\linewidth]{imgs/ADE_val_00000301_qvga_pred_labels_palette.png}
%         & \includegraphics[width=0.31\linewidth]{imgs/ADE_val_00000420_qvga_pred_labels_palette.png} \\
%         (a) & (b)  & (c)
%     \end{tabular}
%     \begin{tabular}{c@{\hspace{2mm}}c}
%          \includegraphics[width=0.48\linewidth]{imgs/ade_val_1989_playing_field_vs_terrain.jpg} 
%          & \includegraphics[width=0.48\linewidth]{imgs/DJX9emTaOwE2R45b.jpg} \\
%         (d) & (e) 
%     \end{tabular}
%         \begin{tabular}{c@{\hspace{2mm}}c}
%         \includegraphics[width=0.66\linewidth]{imgs/coco_playingfield_vs_terrain_161861.jpg}
%          &  \includegraphics[width=0.33\linewidth]{imgs/nyu_110_desk_vs_counter.jpg} \\
%         (f) & (g) 
%     \end{tabular}
%     \caption{``Stuff'' regions in ``in-the-wild'' scenes often are not easily binned into a single category. However, the pair or even triplet of categories that can be simultaneously equally valid is often scene-dependent, encouraging a top-2/top-3 metric. ``Rock'' or ``vegetation'' are appropriate for the mossy boulders (a). [\textcolor{blue}{Traincar restaurant. ``train'' or ``building'' are both appropriate (b).} ``Bookshelf'' or ``shelf'' (or even ``book'') are appropriate for pixels on the right (c). ``Playing field'' or ``terrain'' are both appropriate (d). \textcolor{blue}{``Traffic island'' or ``terrain'' are both appropriate for the area dividing the road (d).} \textcolor{blue}{``Playing field'' or ``terrain'' are appropriate for the grass tennis court, yet COCO labels the green, grassy patch ``terrain'', and the worn beige areas as ``playing field'' (e).} NYU labels the store counter as ``desk'', whereas we consider it a ``counter'', as it is attached to the floor (f). \ozan{This figure is not mentioned in th text, I also do not understand what is it saying}}
%     \label{fig:my_label}
% \end{figure}




%\section{Details on the WildDash Model}
%\label{sec:wilddash}
% For the WildDash results we achieved in Table \textcolor{blue}{4} of main text, we train the same PSPNet-50 model with higher resolution images (shorter image side equal to 480 px) of MSeg. We also train the model for longer so that it sees 1.8 million examples from each dataset, instead of 1 million as in all other experiments. 
%Additionally, we use multi-scale testing for generating the prediction maps, with scales $(0.5, 0.72, 1.0, 1.25, 1.5, 1.75)$.
% \section{Experiments }

% \section{Effects of Adding Datasets}
% \label{sec:add}
% We investigate effects of adding datasets one by one in MSeg, on zero-shot transfer to test datasets. We start from the model trained with three most comprehensive datasets (COCO, Mapillary, ADE20K) and add IDD, Cityscapes, NYU and BDD one by one. This experiment is conducted with the lower resolution training images as in main text.

% \begin{table}[ht]
%     \centering
%     \resizebox{\columnwidth}{!}{
%     \begin{tabular}{@{}lccccc@{}}
%   \toprule
%       Train/Test & VOC &  WildDash & CamVid & ScanNet & \textit{h.\ mean} \\
%         \midrule
%         COCO+Mapillary+ADE20K & $69.2$   & $43.1$   & $63.9$   & $34.6$   & $48.7$ \\
%         +IDD & $68.8$   & $45.4$   & $66.8$   & $34.4$   & $49.6$  \\
%         +Cityscapes & $69.0$   & $45.9$   & $68.2$   & $34.3$   & $49.9$  \\
%         +NYU & $69.0$   & $46.8$   & $69.2$   & $35.8$   & $51.1$  \\
%       +BDD (Full MSeg)  & $68.4$   & $47.8$   & $71.0$   & $35.9$   & $51.6$  \\ \midrule
%         % & & & & & \\
%       Self-training  & $70.0$ & -- & $70.7$ & $55.6$  & -- \\
%       \bottomrule
%     \end{tabular}
%     }
%     \vspace{-2mm}
%     \caption{Effects of adding datasets in MSeg (Zero-shot cross-dataset generalization). 
%     }
%     \label{tab:add_datasets}
%     \vspace{-3mm}
% \end{table}
% Table \ref{tab:add_datasets} shows our results. We can see for most datasets (WildDash, CamVid, NYU), the performance is steadily increasing when we incorporate more datasets. The arithmetic mean is also steadily increasing. 


%\textcolor{red}{Add note that adding each individual dataset was helpful in terms of the mean. We investigate effects of adding datasets one by one in MSeg, on zero-shot transfer to test datasets. We find the arithmetic and harmonic mean steadily increases with each addition.}





% \section{Super-Resolution}
% We use Feedback Network \cite{Li19cvpr_FeedBackSuperRes}
% rather than bilinear, 2x, 3x, ADE20K and COCO


% \section{Multi-Label Annotation}
% In LVIS \cite{Gupta19cvpr_LVIS}, pixels often belong to multiple masks, each annotated with a different category. We see three main reasons for this (1) the dual nature of objects (e.g. table being used as desk, monitor and television set) (2) hierarchical objects parts vs. whole object (sofa and cushion, mushroom and pizza, laptop and keyboard) and (3) objects lying on top of each other (bed and quilt, bed and pillow, person and shirt).

% While one could annotate multi-masks per image to overcome this challenge (as PASCAL Context \cite{Mottaghi:cvpr14:context} and LVIS \cite{Gupta19cvpr_LVIS} do) and allow a prediction of any valid category to qualify for full makrks, we note that given a limited number of classes that avoid hierarchical relationships, selecting one \textit{best} category is generally still natural. We provide WordNet \cite{Miller95acm_WordNet} mappings where possible to link MSeg with LVIS \cite{Gupta19cvpr_LVIS}.








% \section{Results when Trained with Higher Resolution}
% \label{sec:fullresablation}
% In the main text, our models are trained with images of shorter side 240 pixel (except the results for the WildDash in Table \textcolor{blue}{4} in the main text). Now we present the results of models trained with a higher resolution -- shorter side 480 pixel (roughly corresponding to the VGA resolution).
% % \zl{Table already put, Text to be added.}

% \begin{table}[ht]
%     \centering
%     \resizebox{\columnwidth}{!}{
%     \begin{tabular}{@{}lccccc@{}}
%   \toprule
%       Train/Test & VOC &  WildDash & CamVid & ScanNet & \textit{h.\ mean} \\
%         \midrule
%         COCO & $\mathbf{73.8}$ & $38.4$ & $53.5$ & $31.2$ & $44.3$ \\
%         Mapillary & $18.8$ & $46.9$ & $\mathbf{78.7}$ & $1.9$ & $6.5$\\
%         ADE20K & $31.3$ & $31.4$ & $47.7$ & $34.8$ & $35.2$\\
%         IDD  & $13.1$ & $32.6$ & $70.4$ & $1.4$ & $4.9$\\
%         Cityscapes & $10.8$ & $16.5$ & $51.7$ & $1.7$ & $5.2$\\
%         NYU & $6.7$ & $0.1$ & $0.3$ & $21.4$ & $0.4$\\
%         BDD & $13.3$ & $47.6$ & $69.1$ & $1.4$ & $5.0$\\
%         \midrule
%       MSeg  & $\mathbf{73.5}$ & $\mathbf{55.5}$ & $75.9$ & $\mathbf{38.0}$ & $\mathbf{56.2}$\\ \midrule
%         % & & & & & \\
%       Oracle  & $\mathbf{75.5}$ & -- & $74.5$ & $59.0$  & -- \\
%       \bottomrule
%     \end{tabular}
%     }
%     \vspace{-2mm}
%     \caption{Semantic segmentation accuracy (mIoU) on MSeg test datasets, trained with higher resolution. (Zero-shot cross-dataset generalization, corresponding to Table \textcolor{blue}{2} in the main text) 
%     % \textit{Top:} performance of models trained on individual training datasets that make up MSeg. \textit{Middle:} the same model trained on MSeg (our result). \textit{Bottom:} for reference, performance of `oracle' models trained on the test datasets. 
%     % Numbers within 1\% of the best are in bold. The rightmost column is a summary measure: harmonic mean across datasets.
%     }
%     \label{tab:resultsontestdatasets_vga}
%     \vspace{-3mm}
% \end{table}

\iffalse
\section{Multi-task Learning Implementation Details}
\label{sec:mgda}
As discussed in the main paper, we apply the Multiple-Gradient Descent Algorithm (MGDA) \cite{NeurIPS2018:Sener:Koltun}, a multi-task learning algorithm, to MSeg.  A common proxy objective in multi-task learning is to minimize a weighted linear combination of per-task losses. The main idea of the Multiple Gradient Descent Algorithm (MGDA) is instead of heuristically setting such weights, at each iteration solve a small subproblem to find the pareto optimal weight setting. In each iteration, a loss function and loss function gradient is evaluated independently for each dataset. A gradient descent direction is obtained as a convex combination of these various loss gradients.

At every training iteration, we use the following protocol.
We use an identical Frank-Wolfe solver as \cite{NeurIPS2018:Sener:Koltun} to find the pareto optimal per-task weights. Given a minibatch of $m$ examples from $n$ datasets, we place the $\nicefrac{m}{n}$ examples from each dataset on a separate GPU process, and compute a per-dataset loss and loss gradients in each process. Each dataset's gradients are stacked into a high-dimensional vector, and all such vectors are gathered and passed to the Frank-Wolfe solver. As discussed above, the descent direction is the convex combination of the various loss gradients, and afterwards a gradient step is applied.


\section{Domain Generalization Implementation Details}
We adapt the domain generalization (DG) technique proposed for the image classification task in \cite{Motiian:2017:ICCV:CCSA} to semantic segmentation as follows: We add no new parameters to PSPNet, but simply add a contrastive loss. Suppose we have a deep network $h(g(X))$, where $g(\cdot)$ is feature extractor, and $h(\cdot)$ is classifier. We feed a minibatch of 128 crops $X$ through $g(\cdot)$, the ResNet backbone of a PSPNet. We then sample $N$ positive pairs of feature map embeddings, each corresponding to an $8 \times 8$ pixel region per feature map location, and $3N$ negative pairs. In our experiments, we set $N=1000$ or $N=100$.

We choose these 4N pairs by first sampling uniformly randomly  from domains, and subsequently sampling uniformly randomly from pixel locations available in each input crop. When $N>1000$ with a batch size of 128, CUDA memory is insufficient to compute the Euclidean distances between embeddings, forcing us to use $N=1000$. In order to determine positive or negative pairs, we downsample the ground truth label map by $8x$ with `nearest' interpolation and then compare the corresponding ground truth semantic class of feature map locations. In such a way, we identify $N$ pairs of embeddings that belong to the same semantic class. As in \cite{Motiian:2017:ICCV:CCSA}, we set $\alpha=0.25$ such that
\begin{equation}
    \mathcal{L}_{CCSA} = (1-\alpha) \cdot \mathcal{L}_C(h \circ g) + 
    \alpha \cdot \mathcal{L}_{SA}(g) + \alpha \cdot \mathcal{L}_S(g).
\end{equation}
%We compute the contrastive loss with push term for different class pairs and pull term for same-class pairs. Push term says if pair elements come from separate classes, push embeddings apart. Pull term says if pair elements come from the same class, pull embeddings together. Let $\alpha$ be the multiplier on the contrastive loss.  Sum losses as $contrastive\_loss \cdot (\alpha)+ cross\_entropy\_loss \cdot (1-\alpha)$. 

Our implementation differs from \cite{Motiian:2017:ICCV:CCSA} in the following ways: (1) We sample pairs on the fly, instead of choosing fixed pairs for each epoch in advance. (2) We sample uniformly randomly an image crop from all domains first, then sample uniformly from pixel locations in each image crop. Finding evenly-balanced pairs from each class would require sampling a very large number of pairs (we observe $10^5$ times more density in the most populous MSeg class vs. the least populous class). (3) We compute classification loss over all pixel locations and the contrastive loss only over sampled pixel locations, whereas \cite{Motiian:2017:ICCV:CCSA} computed classification loss only over sampled pairs. (4) We use SGD with momentum, a standard optimization technique for PSPNet, rather than using Adadelta. (5) We use a ResNet backbone instead of a VGG backbone for the feature extractor.


\begin{figure}
    \centering
    \begin{tabular}{@{}c@{}c@{}}
        \includegraphics[trim=30 30 30 30, clip,width=0.49\columnwidth]{imgs/universal_px_percentages-qvga-canonical-order-barh_widthpt6_fontsz8_800dpi.png} & \includegraphics[trim=30 30 30 1, clip,width=0.49\columnwidth]{imgs/universal_px-counts-log-scale-qvga-barh_widthpt6_fontsz8.png} \\
        (a) & (b) 
    \end{tabular}
    \caption{(a) Percentage of total number of class pixels from each dataset at \textbf{QVGA resolution}. Classes are ordered from highest to lowest pixel count in MSeg. %\textbf{Top:} 
     \textbf{At QVGA resolution}, COCO Panoptic contributes a large majority of pixels when using a common resolution (e.g. QVGA) because it includes more images than any other dataset.
    (b) Distribution and pixel counts of MSeg classes, in log scale, at  QGA resolution. 
    }
    \label{fig:universal-dataset-class-contributions}
\end{figure}
\fi
