# Supplementary material for: MSeg: A Composite Dataset for Multi-domain Semantic Segmentation
Source: arXiv:2112.13762 source file (2021-12-27)
Supplement: Supplementary file 2 [file appendix_abstract.tex]

In this Appendix, we provide the additional details and additional experimental results we omitted in the main text. In Section \ref{sec:msegadditionaldetails}, we provide additional details regarding MSeg taxonomy. In Section \ref{sec:excludeddatasets}, we provide a discussion of component datasets currently excluded from MSeg. In Section \ref{sec:mturkinterface}, we provide examples of our re-labeling interface and a depiction of our re-labeling workflow. In Section \ref{sec:fullablation}, we provide results of the controlled experiments on the full MSeg dataset. In Section \ref{sec:fullresablation} we provide our main results in the paper with models trained using higher resolution images. Section \ref{sec:wilddash} provides more details on the model trained to achieve state-of-the-art on WildDash datasets.   Section \ref{sec:mgda} compares the MGDA \cite{NeurIPS2018:Sener:Koltun} algorithm for multi-task learning with our strategy of evenly mixing data. Finally, in Section \ref{sec:classdefinitions}, we provide visual examples of every MSeg class.
  
  % Section \ref{sec:add} analyzes the effects of adding each dataset in MSeg.
